# Supplementary material for: DanceText: A Training-Free Layered Framework for Controllable Multilingual Text Transformation in Images
Source: arXiv:2504.14108 source file (2025-09-26)
Supplement: Supplementary file 1 [file x_appendix.tex]

% \appendix

% \section*{Ethical Statement}

% There are no ethical issues.

% \section*{Acknowledgments}

% Acknowledgments

\onecolumn

\clearpage
\newpage
\appendix

\setcounter{page}{1}
\setcounter{section}{0}
\setcounter{table}{0}
\setcounter{figure}{0}

% \maketitlesupplementary

\section{Comparison with Adjustment Methods}  
\label{sec_composition_method}

We compare our depth-aware method with three widely used brightness and contrast adjustment techniques:

\paragraph{Linear Scaling}  
A basic linear adjustment is applied uniformly across the entire foreground without considering depth:

\begin{equation}
I'_{\text{fg}} = \gamma \cdot I_{\text{fg}} + \delta
\end{equation}
where \( \gamma \) and \( \delta \) are fixed scaling factors. This method does not adapt to variations in scene illumination.

\paragraph{Gamma Correction}  
Gamma correction applies a nonlinear transformation to enhance details in dark or bright regions:

\begin{equation}
I'_{\text{fg}} = I_{\text{fg}}^\gamma
\end{equation}
where \( \gamma \) controls the intensity adjustment. While this method improves local contrast, it does not consider spatial variations, often leading to mismatches in illumination.

\paragraph{Histogram Matching}  
Histogram-based methods adjust the brightness distribution of the foreground to match the background:

\begin{equation}
I'_{\text{fg}} = H_{\text{match}}(I_{\text{fg}}, I_{\text{bg}})
\end{equation}
where \( H_{\text{match}} \) represents the histogram transformation function. However, this approach assumes a global match and does not handle spatially varying lighting conditions effectively.

\section{Depth-Aware Adjustment}
\label{sec_hyperparameters}

To ensure photometric consistency between the transformed foreground and the reconstructed background, we introduce a \textbf{Depth-Aware Adjustment} module. This module adaptively modifies the brightness and contrast of the foreground layer based on its alignment with the surrounding depth map, thereby enhancing the realism of text reintegration under diverse lighting and geometric contexts.

\subsection{Mathematical Definition}

Let \( D \in \mathbb{R}^{H \times W} \) be the depth map estimated from the inpainted background in Stage~2, and let \( D_{\text{fg}} \) be the depth of the transformed foreground layer. The pixel-wise difference \( \Delta D = D - D_{\text{fg}} \) captures the spatial misalignment between the foreground and background.

To minimize this mismatch perceptually, we define an appearance adjustment function \( \mathcal{F} \), which adjusts the foreground intensity as:

\begin{equation}
I'_{\text{fg}}(x,y) = \alpha(\Delta D(x,y)) \cdot I_{\text{fg}}(x,y) + \beta(\Delta D(x,y)),
\end{equation}
where the contrast and brightness modulation functions are:

\begin{equation}
\alpha(\Delta D) = 1 + \lambda_1 \cdot \Delta D, \quad \beta(\Delta D) = \lambda_2 \cdot \Delta D.
\end{equation}

Here, $\lambda_1$ and $\lambda_2$ are tunable hyperparameters controlling contrast and brightness sensitivity, respectively. When both are set to zero, the module acts as an identity mapping and no adjustment is applied. This serves as a baseline in our ablation study to evaluate the necessity of depth-guided modulation.

\subsection{Hyperparameter Settings}

\begin{table}[ht]
    \centering
    \caption{Hyperparameter settings for depth-aware adjustment.}
    \begin{tabular}{c|c|c|c}
    \toprule
    \textbf{Hyperparameter} & \textbf{Description} & \textbf{Default} & \textbf{Range} \\ \midrule
    $\lambda_1$ & Contrast adjustment factor & 0.5 & $[0.1, 2.0]$ \\
    $\lambda_2$ & Brightness adjustment factor & 0.3 & $[0.05, 1.0]$ \\
    $\Delta D$ & Depth difference ($D - D_{\text{fg}}$) & Computed dynamically & -- \\
    \bottomrule
    \end{tabular}
    \label{table_depth_aware_params}
\end{table}

\subsection{Tuning Principles}

\noindent
\textbf{Large $\lambda_1$}: Enhances contrast response to depth misalignment, but may cause overshooting or dark halos.\\
\textbf{Small $\lambda_1$}: Leads to weaker contrast modulation, possibly under-emphasizing depth cues.\\
\textbf{Large $\lambda_2$}: Introduces strong brightness variation, potentially causing over/under-exposure.\\
\textbf{Small $\lambda_2$}: Results in minimal brightness change, less effective in high dynamic range regions.

\subsection{Recommended Values by Scene Type}

\noindent
\textbf{Uniform lighting:} $\lambda_1 = 0.3$, $\lambda_2 = 0.2$\\
\textbf{High variation lighting:} $\lambda_1 = 1.0$, $\lambda_2 = 0.5$\\
\textbf{High dynamic range scenes:} $\lambda_1 = 1.5$, $\lambda_2 = 0.8$\\
This depth-aware mechanism enables the foreground text to perceptually blend into scenes of varying complexity, by locally adapting to geometric context and illumination structure. Empirical results in Section~\ref{table_ablation_depth_aware} confirm that it improves both quantitative and perceptual metrics.

\section{Figures}
\label{sec_figs_tables}

\noindent
1. Comparison of different text-to-image generation methods is shown in Figure~\ref{fig_compare_generated} and \ref{fig_compare_generated2}.\\
2. Comparison of different depth estimation methods is shown in Figure~\ref{fig_compare_depth}.

% appendix
% fig_compare_generated
\begin{figure*}[!ht]
    \centering
    \includegraphics[width=1\linewidth]{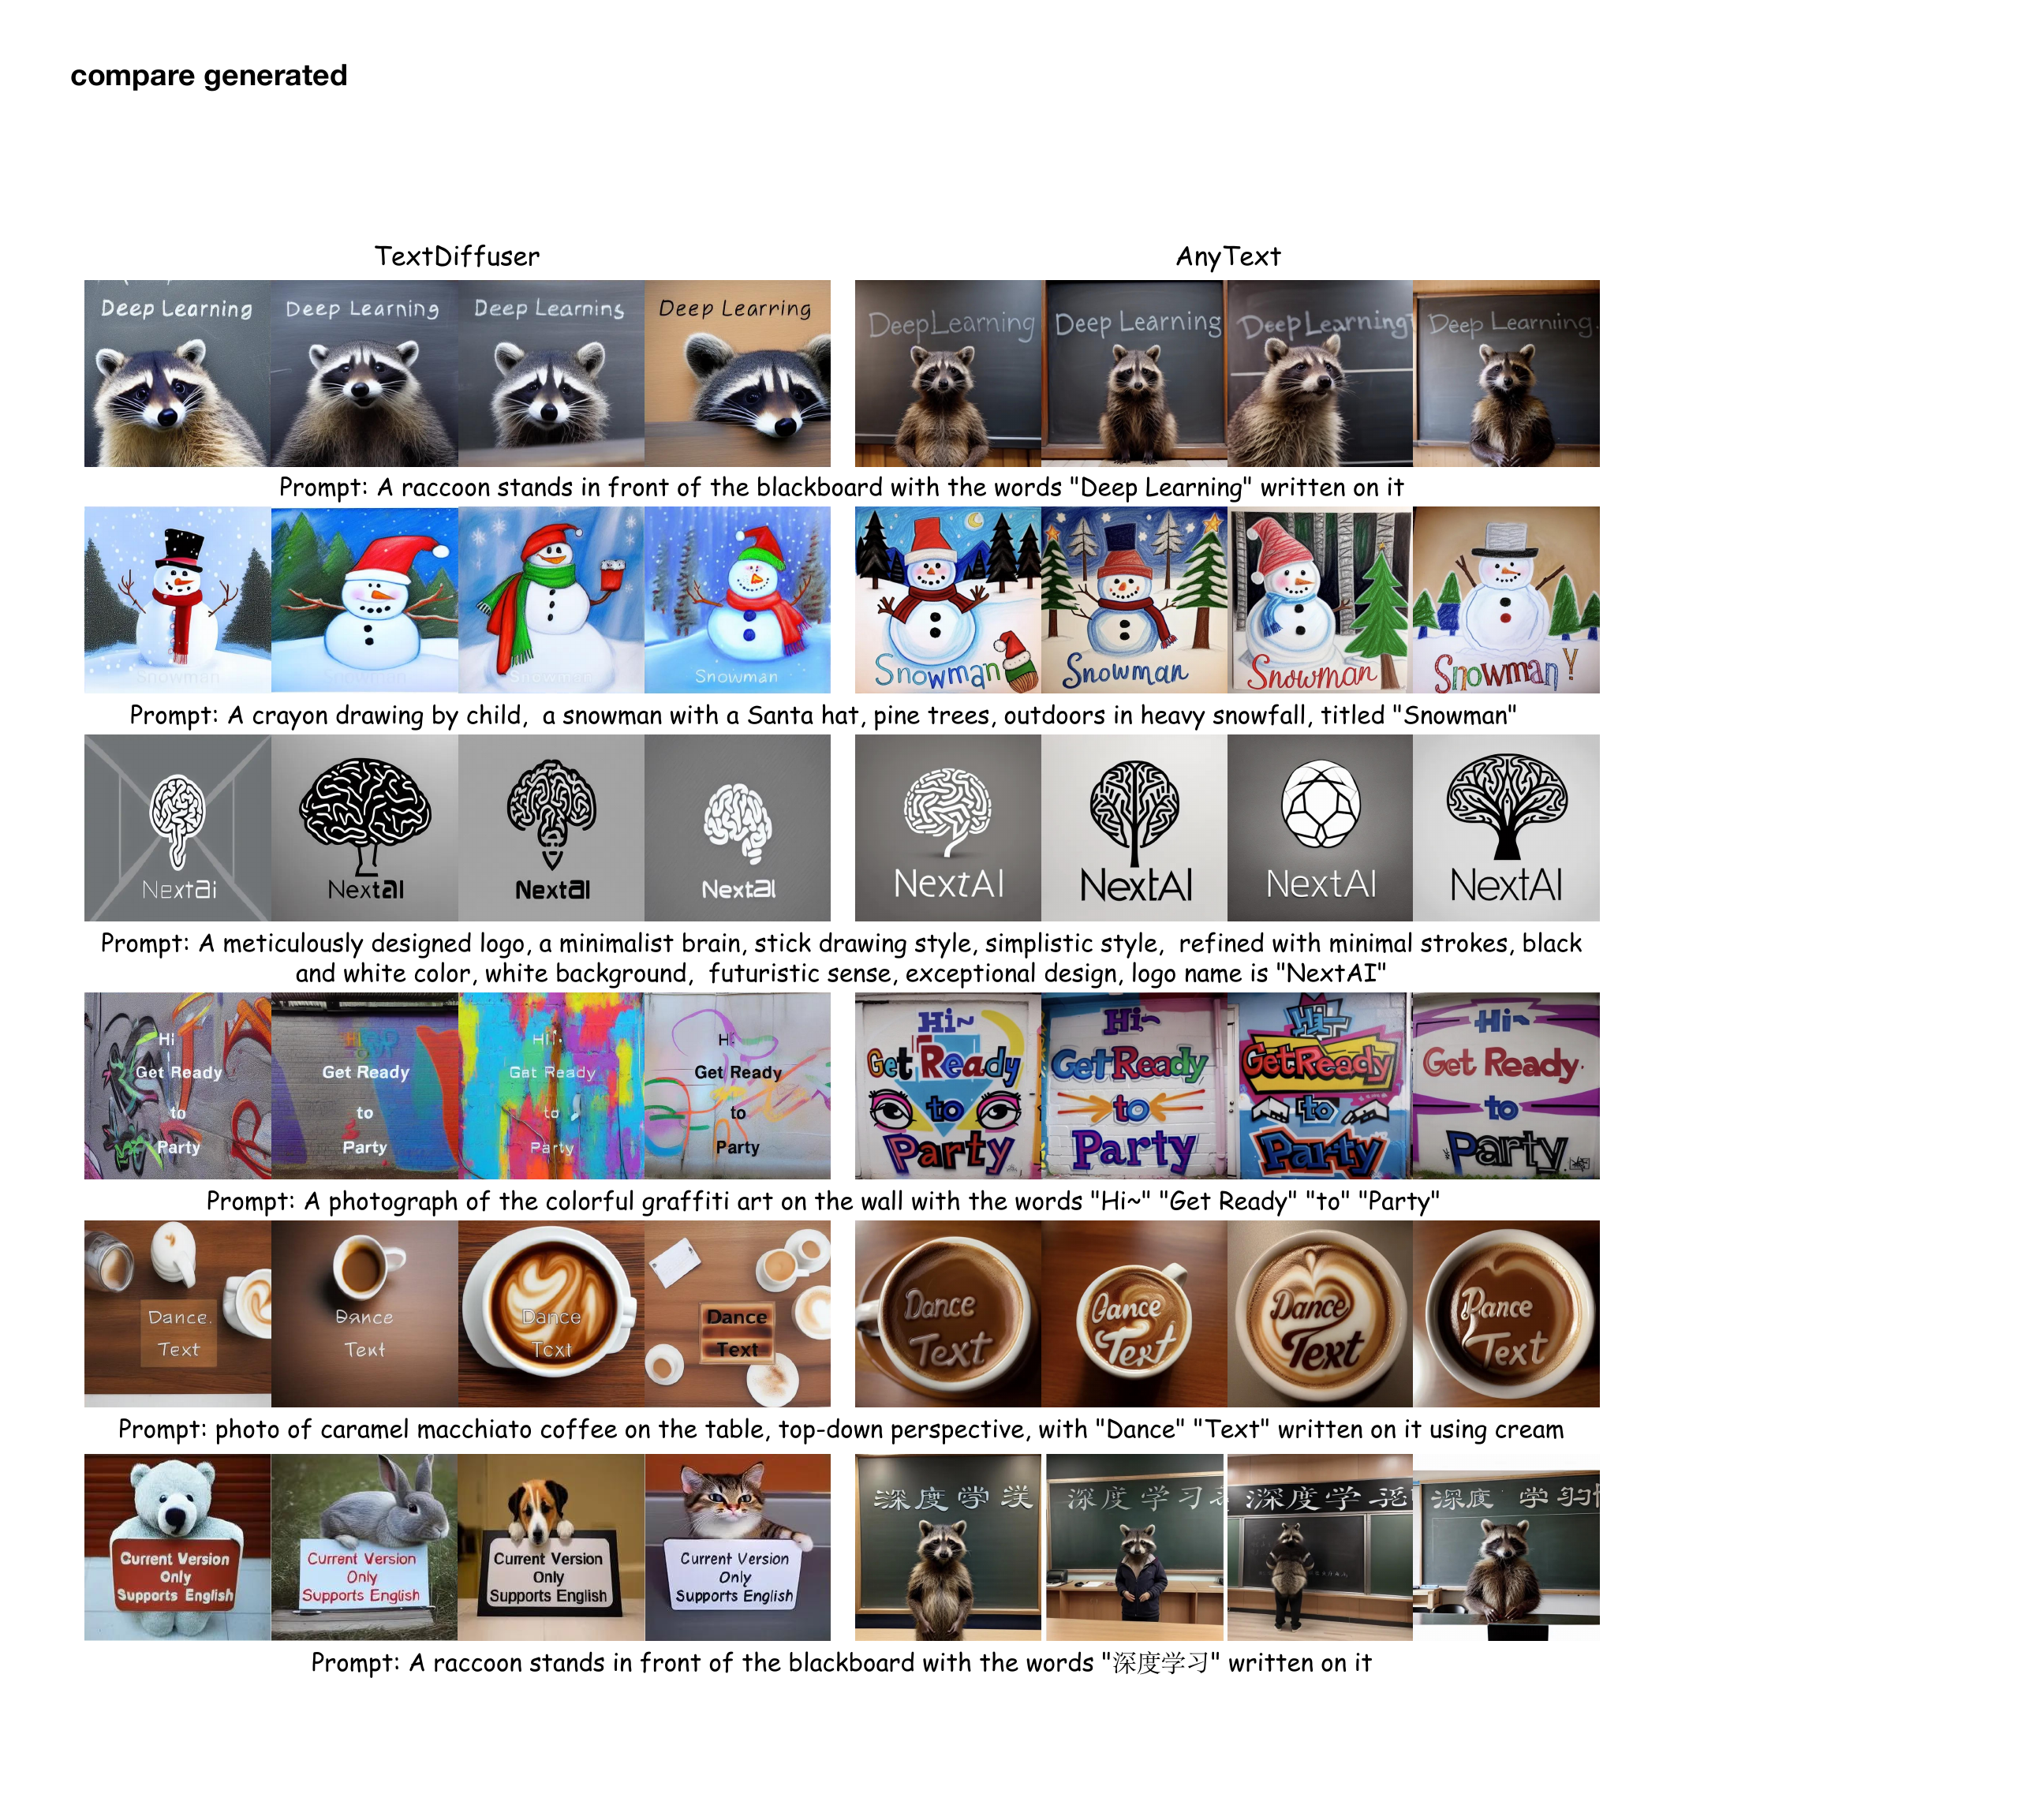}
    \caption{Comparison of different text-to-image generation methods (a). The generative models include \textbf{TextDiffuser}, \textbf{AnyText}, \textbf{Stable Diffusion V1.5, V2.1, V3.0, V3.5}, and \textbf{DALLE}. The comparison highlights differences in text rendering quality, visual coherence, and adaptability across various text editing and generation scenarios.}
    \label{fig_compare_generated}
\end{figure*}

% fig_compare_generated2
\begin{figure*}[!ht]
    \centering
    \includegraphics[width=1\linewidth]{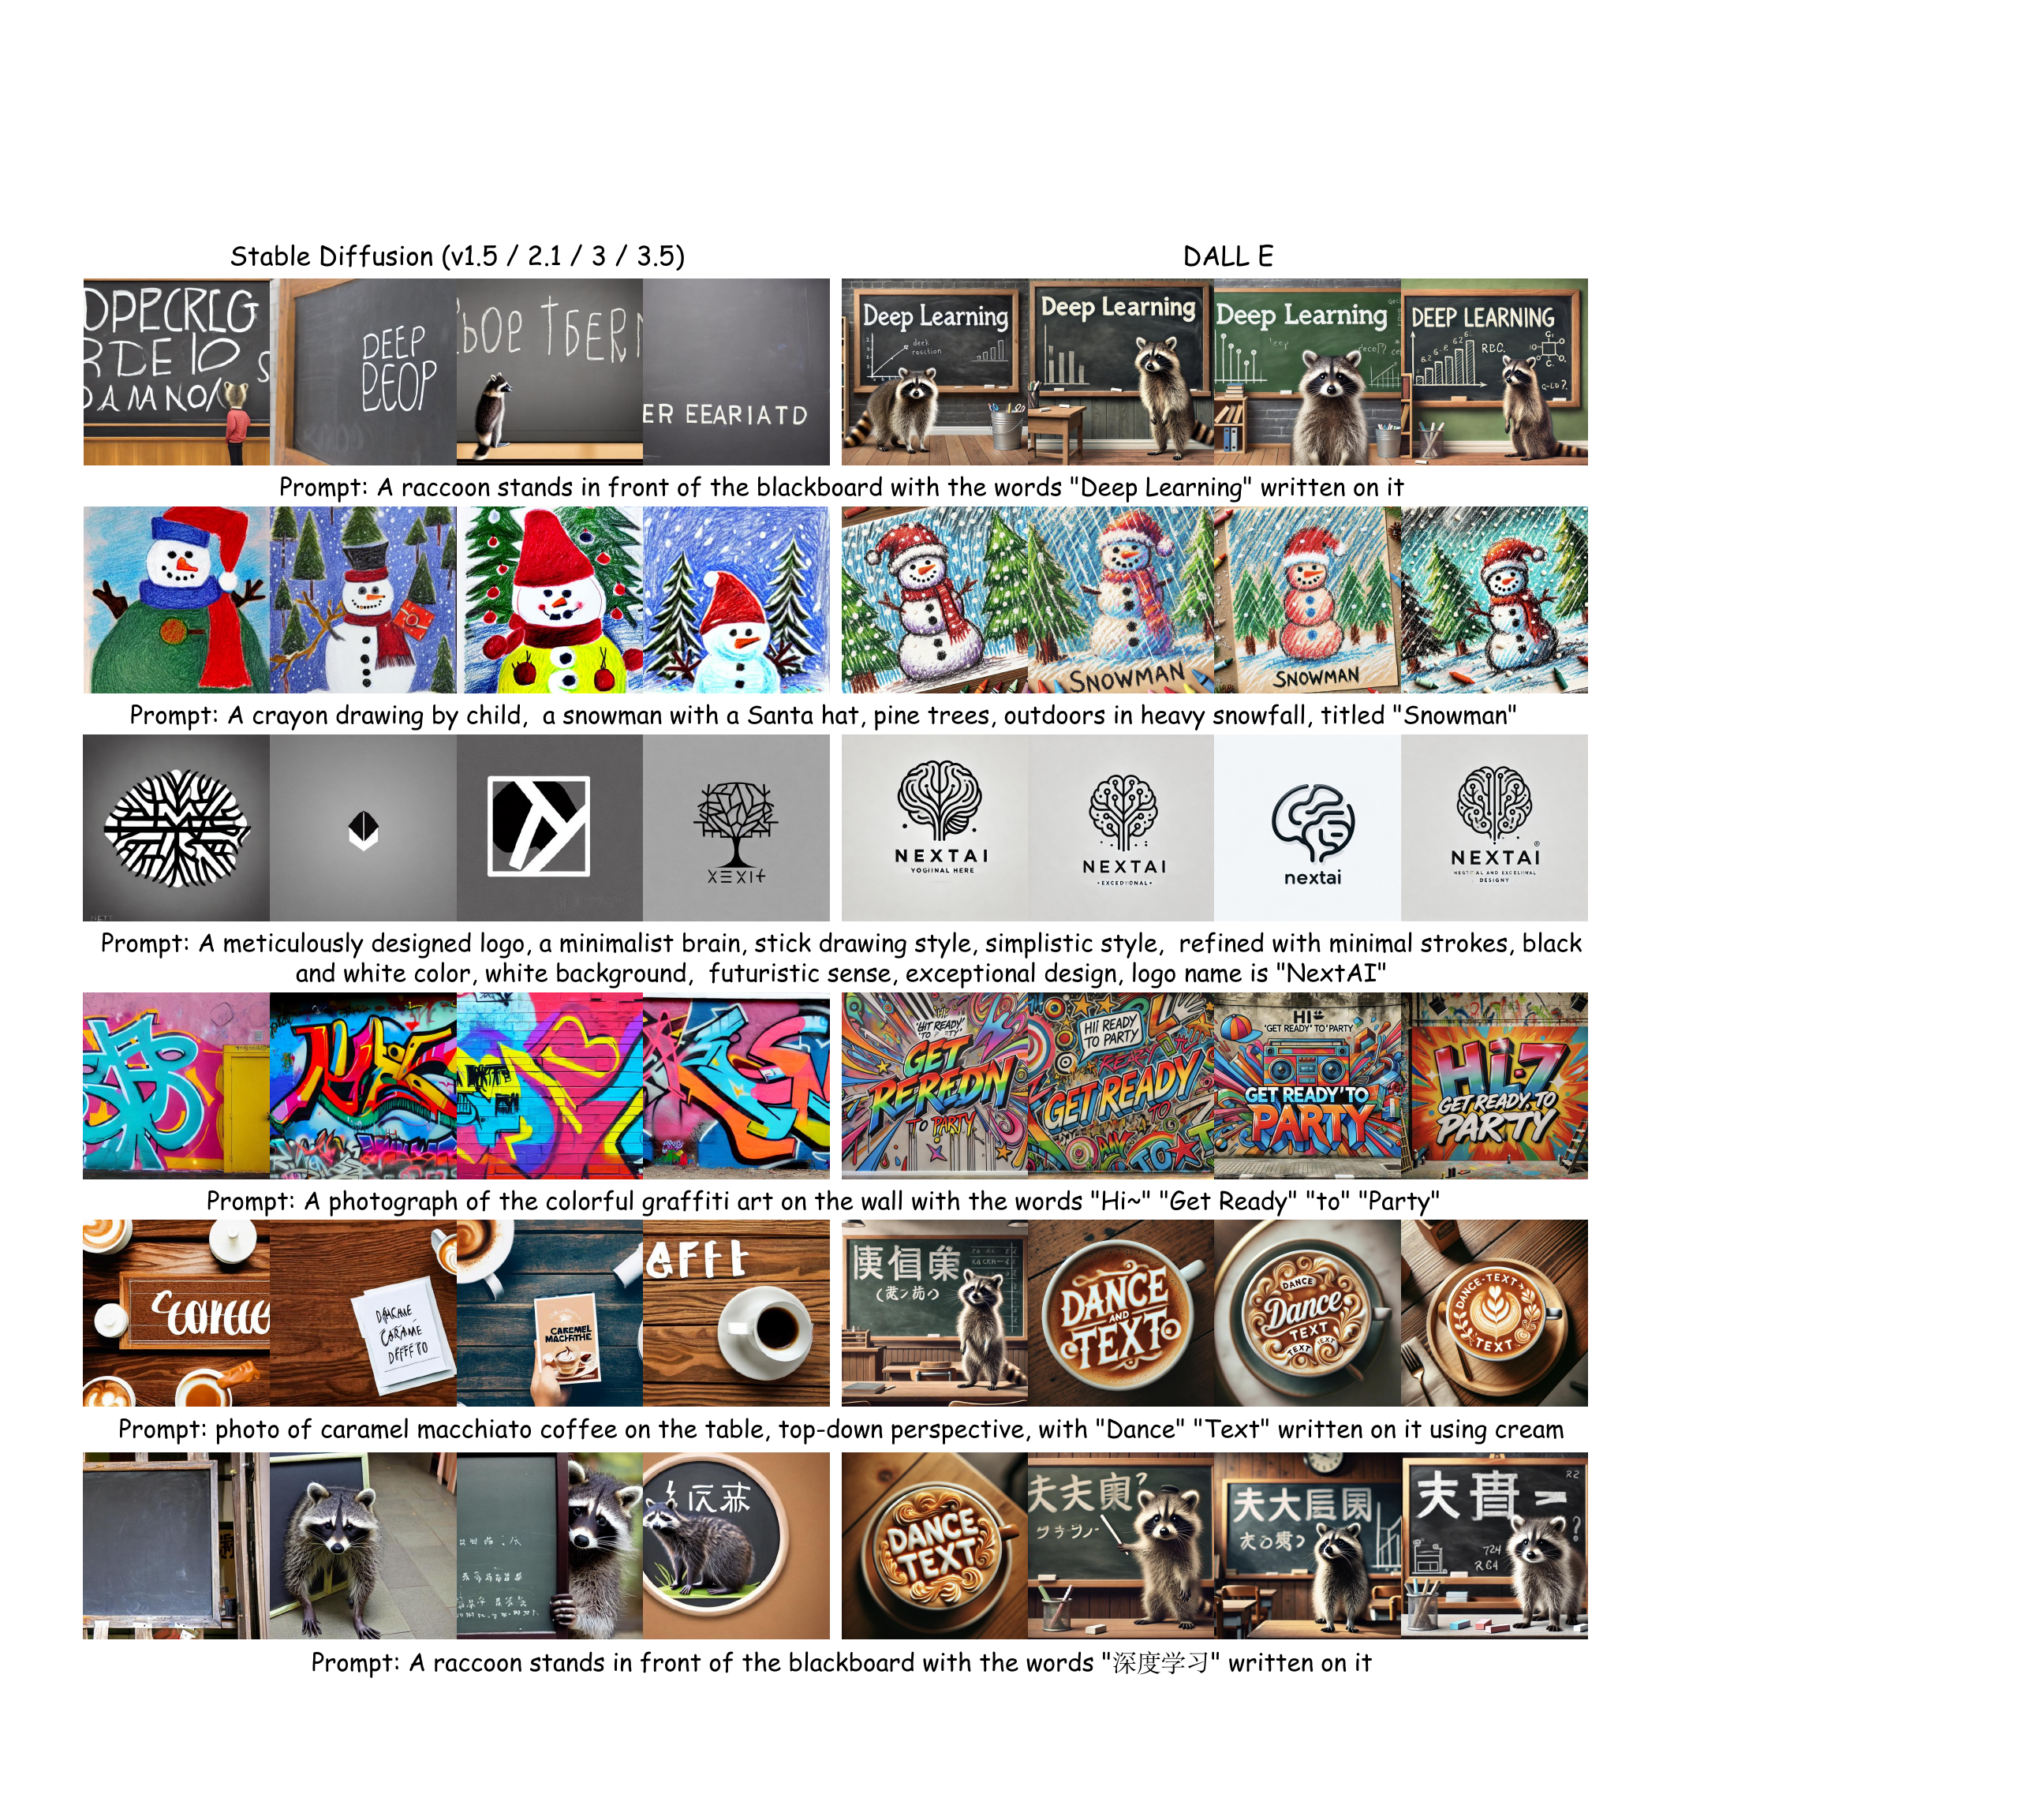}
    \caption{Comparison of different text-to-image generation methods (b). The generative models include \textbf{TextDiffuser}, \textbf{AnyText}, \textbf{Stable Diffusion V1.5, V2.1, V3.0, V3.5}, and \textbf{DALLE}. The comparison highlights differences in text rendering quality, visual coherence, and adaptability across various text editing and generation scenarios.}
    \label{fig_compare_generated2}
\end{figure*}

% appendix
% fig_compare_depth
\begin{figure*}[!ht]
    \centering
    \includegraphics[width=1\linewidth]{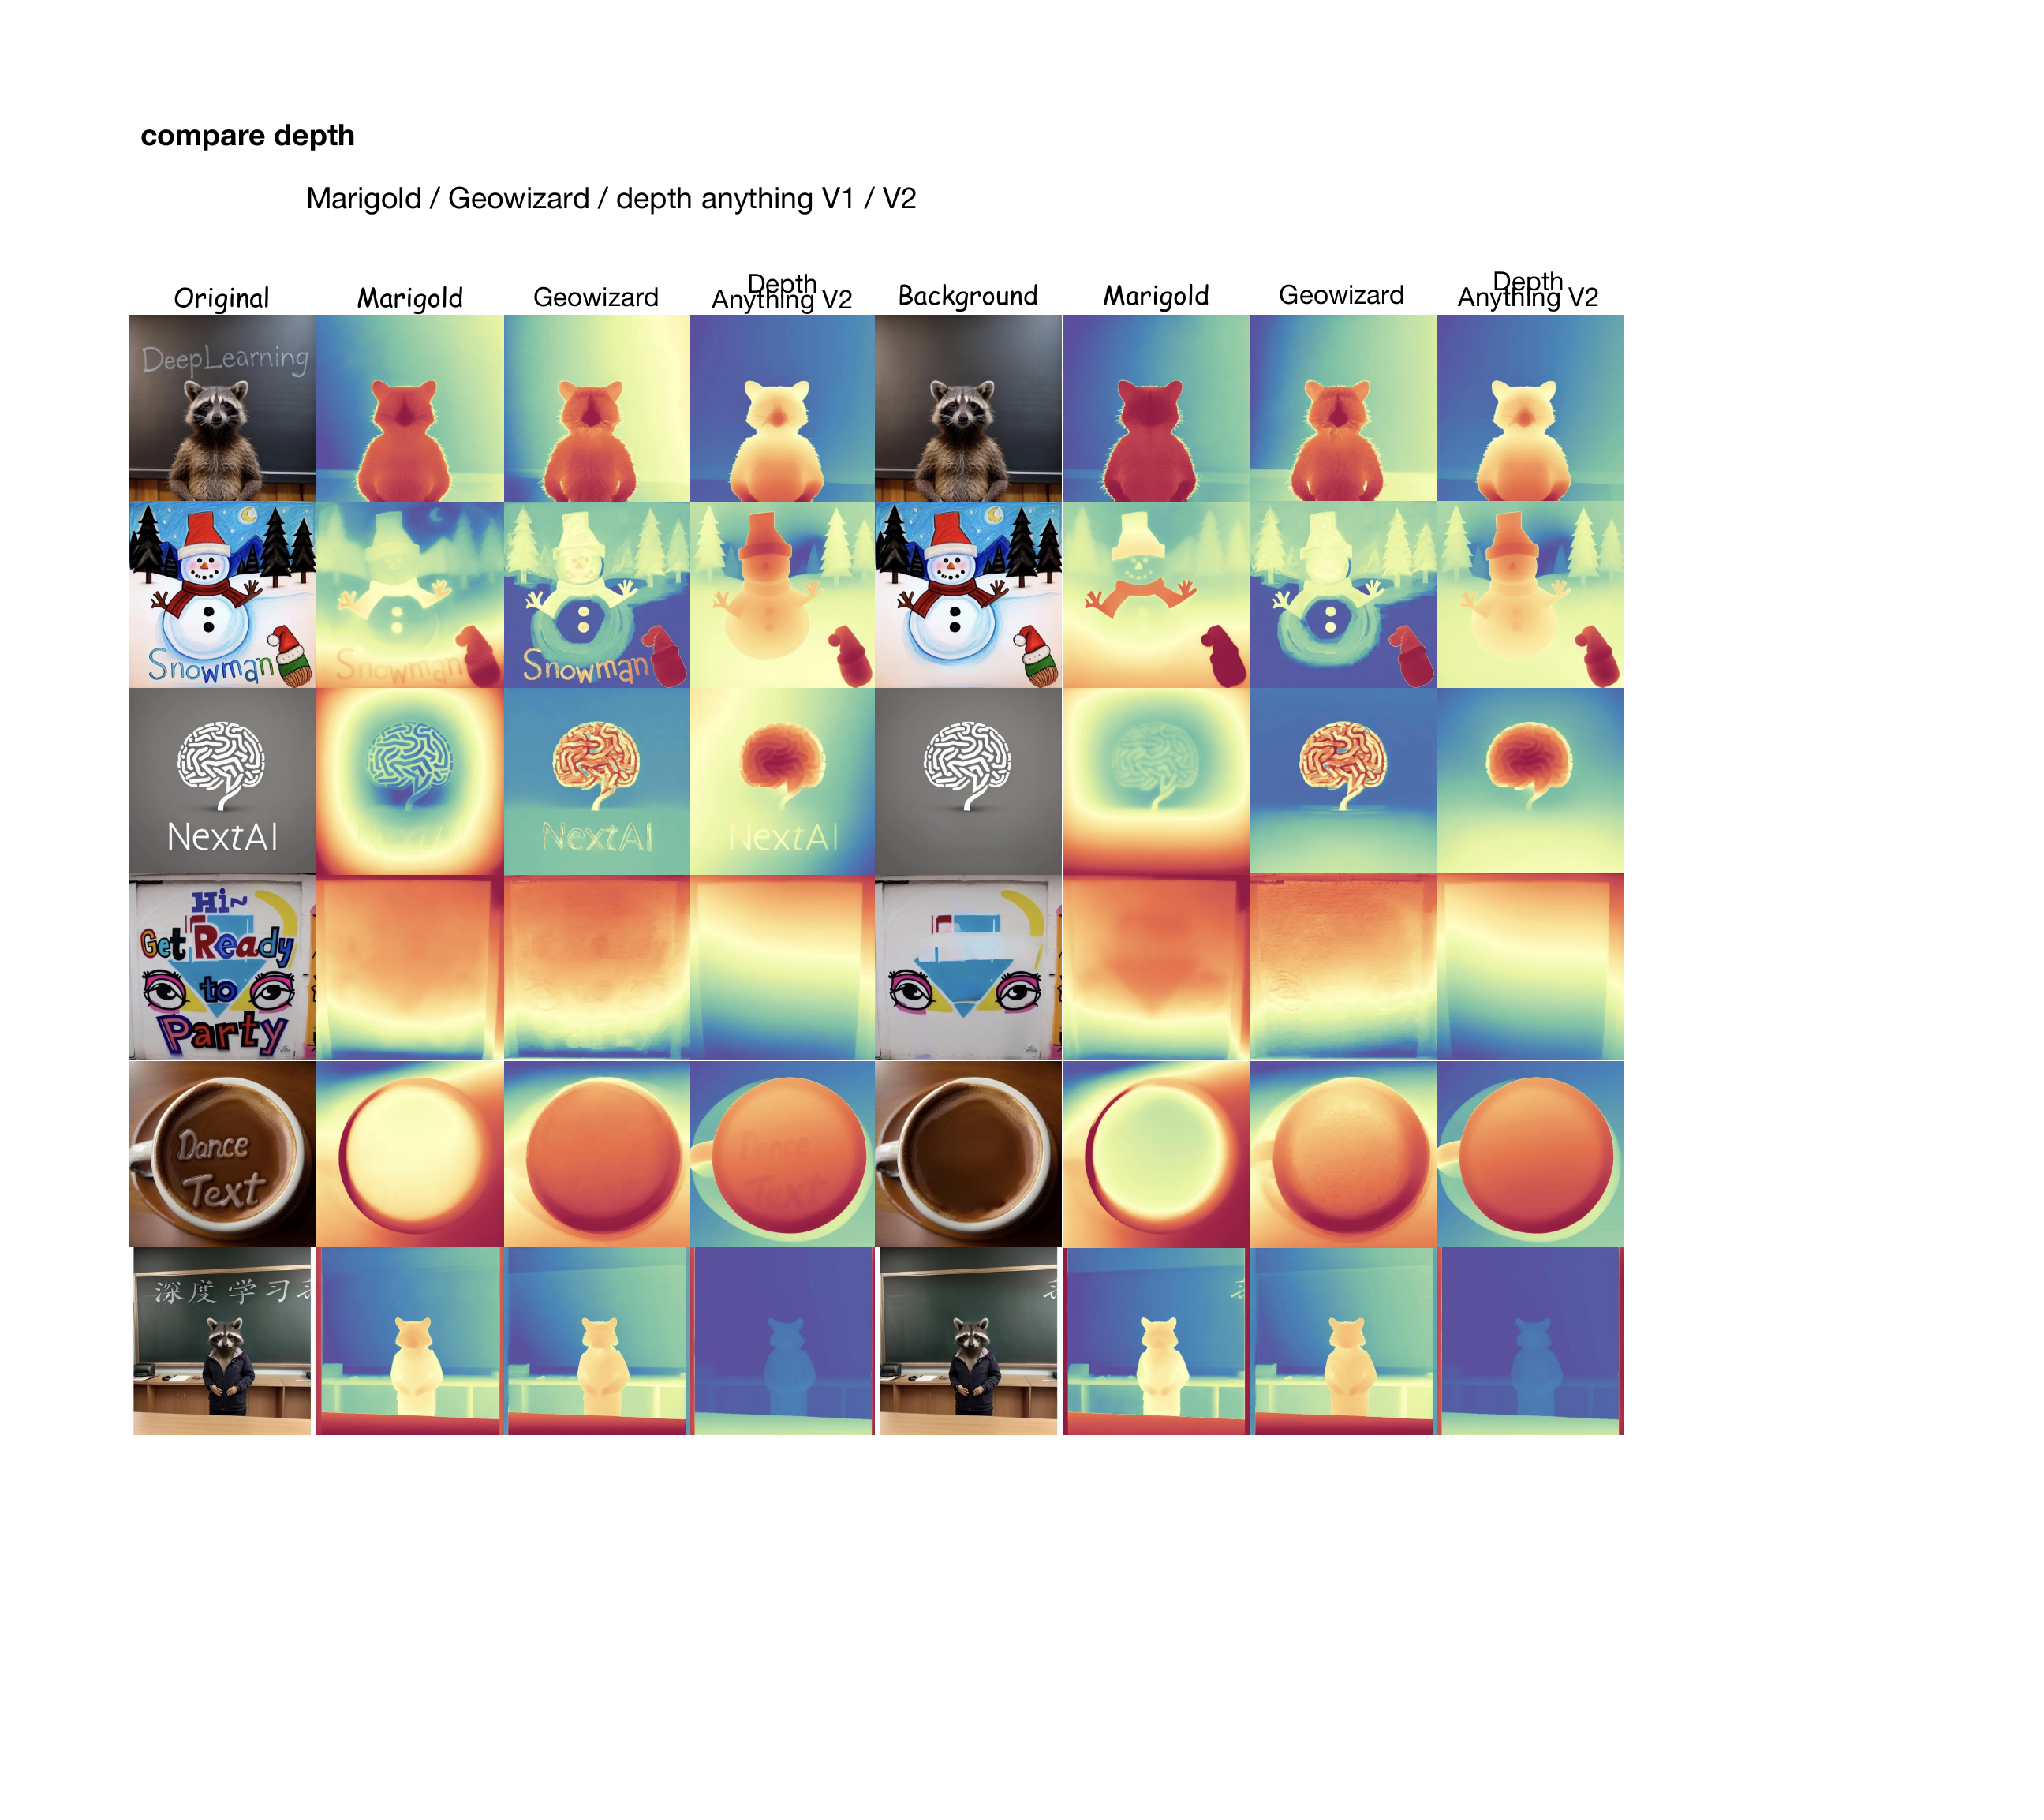}
    \caption{Comparison of different depth estimation methods. The methods include \textbf{Marigold}, \textbf{Geowizard}, and \textbf{Depth Anything V2 (DAv2)}. We selected \textbf{DAv2} as the final depth estimation method due to its better stability and enhanced robustness across various scenes.}
    \label{fig_compare_depth}
\end{figure*}
